# Supplementary material for: Coloring a Dominating Set Without Conflicts: q-Subset Square Coloring
Source: arXiv:2303.06864 source file (2023-03-13)
Supplement: Supplementary file 1 [file appendix.tex]

%\section{Bounds on the number of colors for \SH coloring}

\noindent
Let us familiarize ourselves with \SH coloring with the help of some classes of graphs. We present the upper bound on the number of colors required to \SH color these graph classes. The graphs that we study include complete graph, path, cycle, threshold graph and trees. These are followed by bounds on the number of colors used to color graph $G$ when we consider certain graph parameters such as maximum degree of $G$, size of vertex cover of $G$, cluster vertex deletion number and modular width of $G$.

\subsection{Bounds for \SH coloring with respect to some classes of graphs}

\begin{definition}
Consider a graph $G$ on $n$ vertices. A complete graph $K_n$ is a graph $G$ on $n$ vertices with an edge between any two vertices $u,v \in V(G)$.
\end{definition}

\noindent
Let us analyse the number of colors required to \SH color a complete graph $K_n$.

\begin{lemma}\label{completeG}
If G is a complete graph on n vertices then $\chi_{ssc}(G) = 1$.
\end{lemma}

\begin{proof}
The graph $K_n$ has each vertex adjacent to every other $n - 1$ vertices in the graph. Therefore, by assigning a color to any one vertex of the graph will ensure that each vertex $v \in K_n$ is adjacent to the vertex that is assigned a color. So this gives us a \SH coloring of $K_n$ such that $\chi_{ssc}(G) = 1$.
\end{proof}
\begin{corollary}
If a graph $G$ with a vertex $v$ which has an edge between each vertex $u \in G$, then $\chi_{ssc}(G) = 1$. Examples of such graphs are wheel graph ,flower graph, double wheel graph,etc.
\end{corollary}

\begin{lemma}\label{pathG}
If $G$ is a path on n vertices then $\chi_{ssc}(G) = 1$.
\end{lemma}
\begin{proof}
Any path on $n$ vertices requires exactly one color to be \SH colored. We give a constructive proof of this. Consider a path $P_n$ such that it has $3k$ or $3k + 2$ vertices where $k \geq 1$. We can color every third vertex beginning from the second vertex from one of the end vertices of the path. For path of length $3k+1$, we can color the first vertex using color 1 and every third vertex using the same color and so on. This ensures that every vertex is dominated by exactly one colored neighbor in its closed neighborhood.
\end{proof}

\begin{lemma}
If G is a cycle on $3n$ vertices then $\chi_{ssc}(G) = 1$. Further, if G is a cycle on $3n + 1$ or $3n + 2$ vertices then $\chi_{ssc}(G) = 2$.
\end{lemma}
\begin{proof}
For a cycle on $3n$ vertices, we color every third vertex and hence get a \SH coloring using 1 color. For cycles on $3n+1$ and $3n+2$ vertices, we use color 1 to color every third vertex beginning from a vertex, say $v_1$, and finally use color 2 to color the last vertex that appears in this sequence.

Furthermore, we note that one color is not sufficient for cycles on $3n + 1$ or $3n + 2$ vertices. Consider a cycle on $3n+1$ vertices. To \SH color this cycle using one color, we start by coloring vertex $v_1$ and assign the same color to every third vertex. We observe that the vertex $v_n$ is also assigned the same color as $v_1$, which does not \SH color vertices $v_1$ and $v_n$. Therefore, to avoid this conflict, we color vertex $v_n$ using a new color. Now consider a cycle on $3n+2$ vertices. We color the vertices using one color, as it was done for cycles on $3n+1$ vertices. We observe that vertices $v_1$ and $v_{n-1}$ of the cycle on $3n+2$ vertices are colored using the same color. So, to dominate vertex $v_n$, we assign it a new color. Therefore, for cycles on $3n+1$ and $3n+2$ vertices, we have $\chi_{ssc}(G) = 2$.
\end{proof}

\begin{definition}
A graph is a lollipop graph if it consisting of a complete graph with $m$ vertices and a path $P_n$, where end vertex of path is attached to one of the vertex in the complete graph.
\end{definition}

\begin{lemma}
If G is a lollipop graph $(G)$ then $\chi_{ssc}(G) = 1$.
\end{lemma}

\begin{proof}
From the lemma \label{completeG}, chromatic number of complete graph is one. 
Consider a path $P_n$ which is connected to complete graph at vertex $v$, such that it has $3k + 2$, $3k + 1$ vertices where $k \geq 1$. We can color the vertices on $P_n$, as same as proof given in the lemma \label{pathG}. Since first vertex in the $P_n$ is colored, every vertex in the complete graph is dominated by the first vertex in $P_n$. 
If $P_n$ has $3k$ vertices where $k \geq 1$, then we can color every third vertex beginning from the end vertices of the path. All the vertices in the complete graph and the first vertex in $P_n$ are dominated by any vertex other than $v$ from the complete graph. This ensures that every vertex is dominated by exactly one colored neighbor in its closed neighborhood.

\end{proof}

\noindent
Now we study the nature of \SH coloring with respect to threshold graphs.

\begin{definition}
\cite{golumbic} A graph is a threshold graph if it can constructed from the empty graph by repeatedly adding either an isolated vertex or a dominating vertex.
\end{definition}

\begin{lemma}
If G is a threshold graph then $\chi_{ssc}(G) = 1$.
\end{lemma}

\begin{proof}
If isolated vertices are present, color them using the same color. By coloring the last introduced dominating vertex $v$, we satisfy \SH color $G$ as each vertex in $G$ has only one colored vertex $v$ in its closed neighborhood.
\end{proof}

\begin{definition}
A graph is a sunflower graph $SF_n$ is a graph obtained by adding triangle on  each edge of the rim of a wheel graph $W_n$, such that two triangles,say petals share a common vertex if and only if the corresponding edges in $W_n$ are adjacent in $W_n$.
\end{definition}

\begin{lemma}
If G is a sunflower graph on $n$ vertices, where $n=odd$ then $\chi_{ssc}(G) = 2$. Otherwise $\chi_{ssc}(G) = 3$.
\end{lemma}

\begin{proof}
If we color the vertex $v$, which has an edge between all vertices on the outer cycle on the $W_n$, Then all vertices on $W_n$ will be dominated by $v$. Since two petals share a vertex, we need exactly two colors and we can alternatively use the colors to dominate all petals. Therefore we need three colors to dominate $SF_n$, where $n$ is even. If we dominate the vertex $v$ by a vertex $u$ from the outer cycle on the $W_n$, then two petals are dominated by $u$,which are share the vertex $u$. We need exactly two colors to dominate all petals. Since we can reuse the color of $u$ for the petals where $u$ is not part of it. Therefore we need only two colors to dominate $SF_n$, where $n$ is odd. If we use the same way of \sh of $SF_n$, where $n$ is even, to dominate the vertex $v$ by a vertex $u$ from the outer cycle on the $W_n$ in $SF_n$, where $n$ is even. Then also we need one more color to dominate the petal, which is adjacent to a petal, where $u$ is part of it. Therefore any possible \sh (either color the vertex $v$ or $u$) of $SF_n$, where $n$ is even needed three colors.
\end{proof}

Now using the similar proof of \SH coloring with respect to sun graphs. Corollary follows, 

\begin{definition}
A graph is a sun graph $SF_n$ is a graph obtained by adding triangle on adjacent vertices of the outer cycle of the complete graph graph $K_n$, such that two triangles,say petals share a common vertex if and only if the corresponding edges in outer cycle of $K_n$ are adjacent in $K_n$.
\end{definition}

\begin{corollary}
\label{sun}
If G is a sun graph on $n$ vertices, where $n=odd$ then $\chi_{ssc}(G) = 2$. Otherwise $\chi_{ssc}(G) = 3$.
\end{corollary}

\begin{definition}
A graph is a grid graph if and only if it is an induced subgraph of a grid 
A two-dimensional grid graph ($m\times n$), also known as a rectangular grid, which is Cartesian product of $P_m$and $P_n$.

\end{definition}

\begin{lemma}
If G is a grid graph then $\chi_{ssc}(G) = 2$.
\end{lemma}

\begin{figure}[htb]
\centering
\includegraphics[scale=0.5]{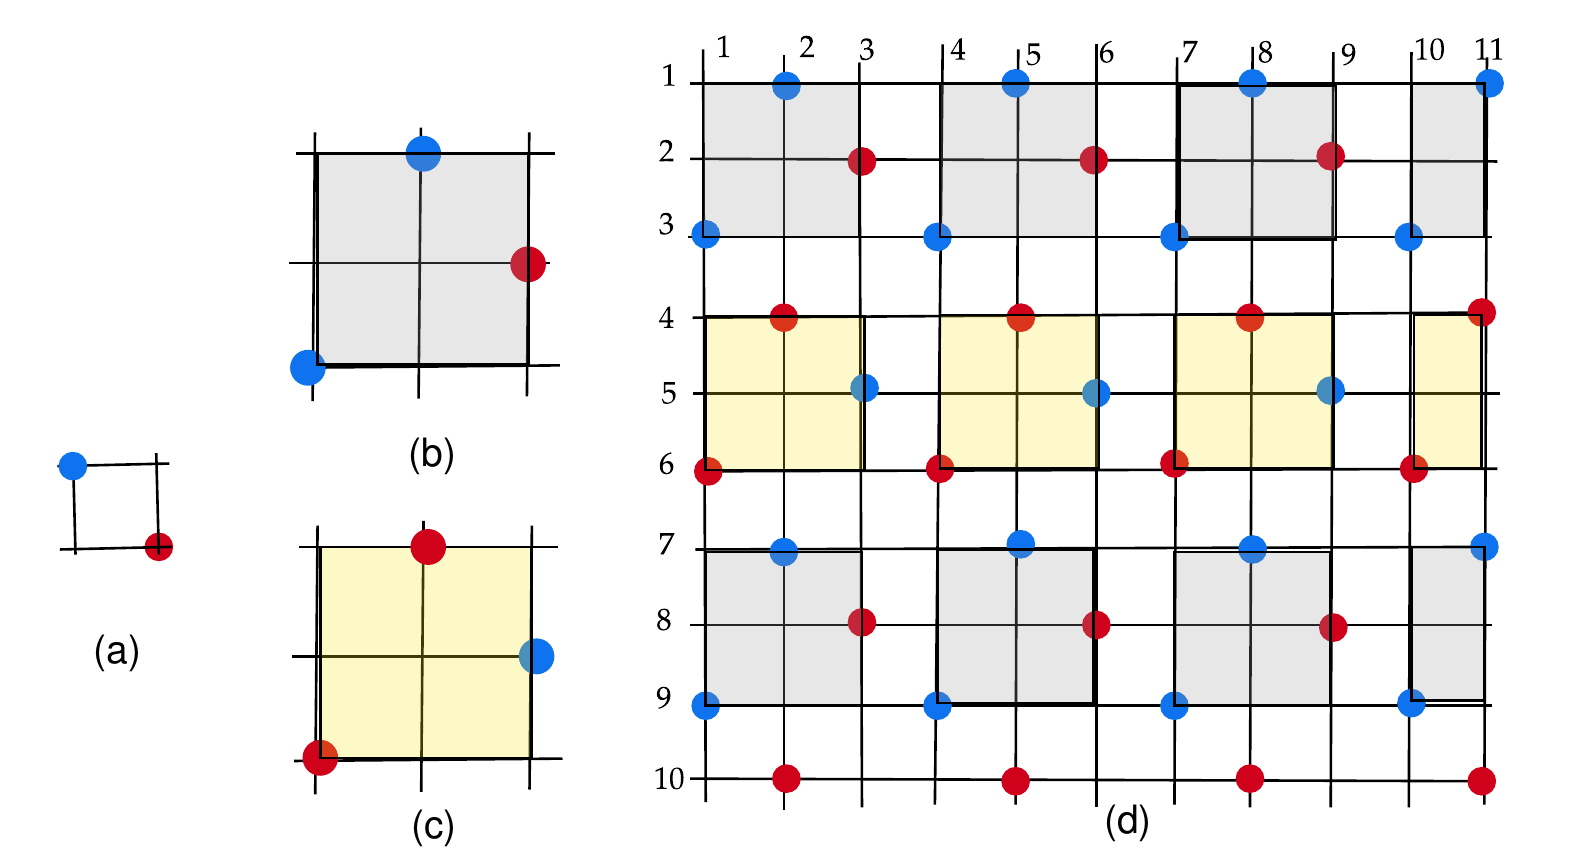}
\caption{\SH coloring using two color on grid graphs}
\label{Figure: grid}
\end{figure}

\begin{proof}
Any grid $1 \times 1$ needs exactly two vertices, shown in figure \ref{Figure: grid}(a). In general, $m \times n$ grid requires exactly two colors in \SH coloring. We give a constructive proof of this. Consider a $3 \times 3$ grid, which can be colored using two colors shown in figure \ref{Figure: grid}(b). This ensures that every vertex is dominated by exactly one of the colored neighbor in its closed neighborhood. For $3k \times 3k$ grid, in every column we repeat the same coloring shown in \ref{Figure: grid}(b). In every row we alternatively use the coloring shown in \ref{Figure: grid}(b) and (c). From this coloring we can observe that paths in the $(3k+1)^{th}$ row and $(3k+1)^{th}$ column in $(3k+1) \times (3k+1)$ grid are self dominated by one color, shown in figure \ref{Figure: grid}(d). Therefore to dominate paths in the $(3k+2)^{th}$ row and $(3k+2)^{th}$column can also be dominated using two colors.

\end{proof}

\begin{definition}
A graph is a grid caterpillar graph if and only if it is a tree having a chordless
path $P_t$ on t vertices, called central path, which contains atleast one
endpoint of every edge. Caterpillar graph is a denoted as $P(n,r_1, r_2,\dots r_n)$, where $r_i$ is the number of pendent vertices attached to $i^{th}$ vertex of $P_n$.
\end{definition}

\begin{lemma}
If G is a caterpillar graph graph then $\chi_{ssc}(G) = 3$.
\end{lemma}

\begin{figure}[htb]
\centering
\includegraphics[scale=0.5]{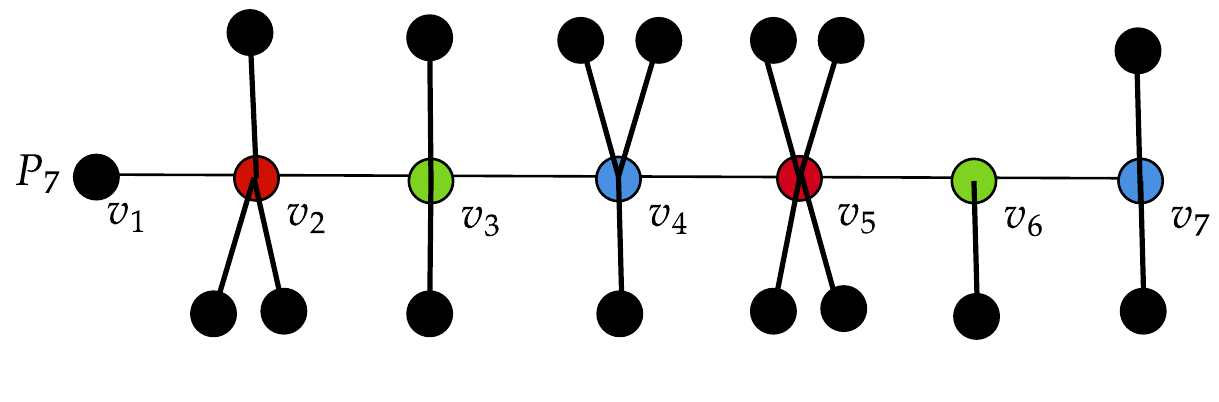}
\caption{\SH coloring using three color on central path in caterpillar graph graphs}
\label{Figure: grid}
\end{figure}

\begin{proof}
If $P(n=3, r_1, r_2, r_3)$, where $r_i \geq 3$ and $\forall r_j=2$, $1 \leq j,i \leq 3$, and $j \neq i$ to dominate all leaves attached to the vertices on the central path, \sh uses different colors to vertices on the central path. Otherwise if we color all leaves of the vertex  $r_i \geq 3$, then we need more than three colors to dominate $r_i$. In general caterpillar graph, we can reuse the three colors of $r_1, r_2, r_3$ for all the vertices on the central path. Therefore $\chi_{ssc}(G) = 3$.

\end{proof}

\begin{definition}
\cite{honeycomb} A honeycomb network
can build from hexagons in various ways. A honeycomb network of size one is a single hexagon,
denoted by $h(1)$. Honeycomb network of
size 2 denoted $h(2)$, can be obtained by
adding six hexagons around the boundary
edges of $h(1)$. In general, honeycomb
network $h(n)$ can be obtained from $h(n –
1)$ by adding a layer of hexagons around the
boundary edges of $h(n – 1)$.
% Alternatively, the size d of HC(n) is determined as the number of hexagons between the center and boundary of HC(n) (inclusive) and the number of vertices and edges of HC(n) are $6n^2$ and $9n^2-3n$ respectively. 
\end{definition}

\begin{lemma}
If G is a honeycomb network of size $h(even)$ or $h(1)$, then $\chi_{ssc}(G) = 1$. Else $\chi_{ssc}(G) = 2$.
\end{lemma}

\begin{proof}
In $h(1)$ we use a color for any two vertices at a distance of 3. For $h(even)$
we color every fourth vertex in a zigzag path from $h(even)$ refer figure \ref{Figure: label_honeyEven}. Furthermore we note that above coloring using one color is not sufficient for $h(odd)$ except $h(1)$ refer figure  \ref{Figure: label_honeyOdd}(d). To dominate $h(1)$, either choose one of the following, 

\begin{enumerate}
\item Two vertices from $h(1)$, they are opposite to each other.
	\begin{enumerate}
	\item There exist four vertices from the outer cycle of $h(3)$ with distance three refer figure \ref{Figure: label_honeyOdd}(b). W.l.o.g consider $p_1$ and $p_2$ from figure \ref{Figure: label_honeyOdd}(b), are at distance two from each other. If we color using first color other vertex can not dominate using a vertex from outer cycle of $h(2)$. Therefore we need to dominated by a vertex from outer cycle of $h(3)$. We use the first color on every end vertex of $P_3$ from the colored vertex. If we continue this we will end up with some vertices which needs one more color refer top of the figure \ref{Figure: label_honeyOdd}(b). 
	\item If we start to dominate the vertices from $h(2)$ by coloring the vertices from outer cycle of $h(2)$. It form a zigzac path and end up with uncolored and undominated vertex, refer figure \ref{Figure: label_honeyOdd}(a).
	\end{enumerate}
\item None of the vertices from $h(1)$

\begin{enumerate}
\item If we color every fourth vertex from  the outer cycle of$h(3)$, refer figure \ref{Figure: label_honeyOdd}(c). We will be left with some vertex on outer cycle of $h(2)$.
\end{enumerate}

\item All vertices from $h(2)$.

\begin{enumerate}
\item If we color every fourth vertex in a zigzag path from $h(2)$, refer figure \ref{Figure: label_honeyOdd}(d). We will be left with some vertex on outer cycle of $h(3)$.
\end{enumerate}

\item One vertex from $h(1)$, remaining from $h(2)$.
\begin{enumerate}
\item If we start to dominate undominated vertex of $h(1)$ by vertices from $h(2)$. We will be left with some vertex on outer cycle of $h(3)$, refer figure \ref{Figure: label_honeyOdd}(e)
\end{enumerate}
\end{enumerate}

\end{proof}

\begin{figure}[htb]
\centering
\includegraphics[scale=0.8]{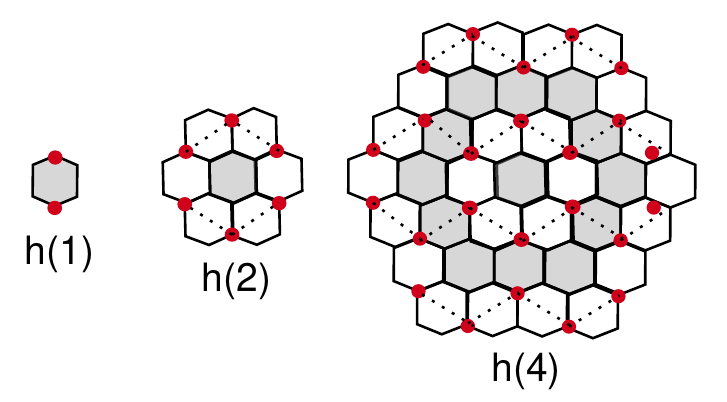}
\caption{\SH coloring using one color $h(even)$ and $h(1)$}
\label{Figure: label_honeyEven}
\end{figure}

\begin{figure}[htb]
\centering
\includegraphics[scale=0.7]{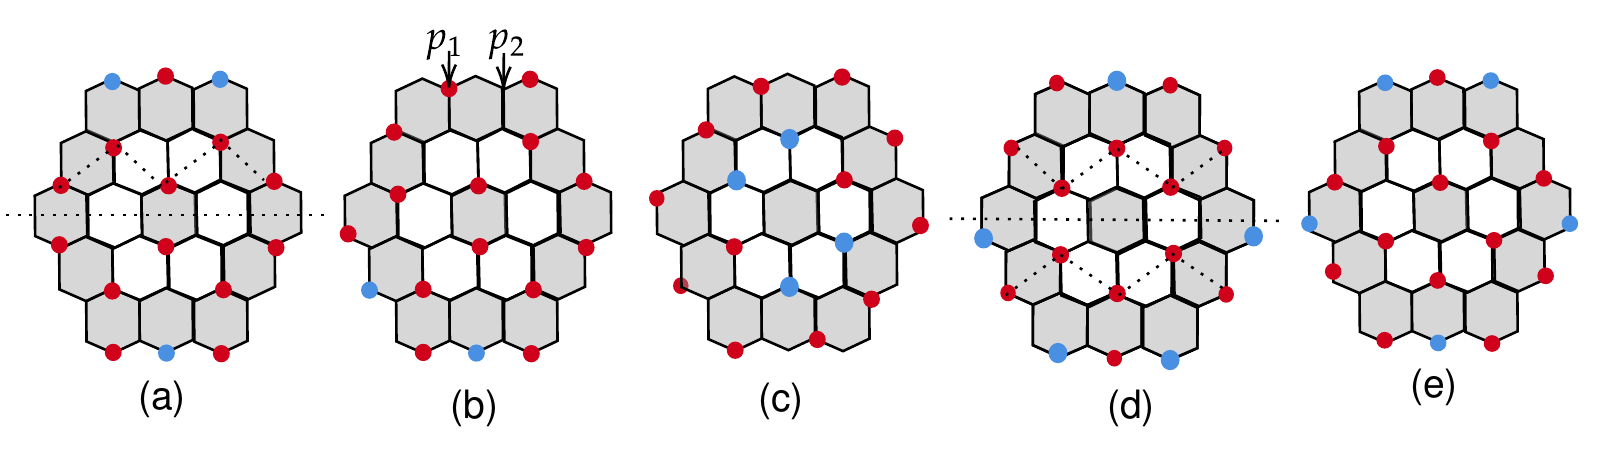}
\caption{\SH coloring using one color $h(even)$ and $h(1)$}
\label{Figure: label_honeyOdd}
\end{figure}

\begin{lemma}\label{treebound}
Let $\Delta$ be the maximum degree of a tree. Then $\Delta$ colors are sufficient to \SH color the tree. Moreover, $\Delta-1$ colors are sometimes necessary.
\end{lemma}
\begin{proof}
Consider a tree $T$ with a root $r$. Color root $r$ with a color $c_i$ where $i \neq 0$. The nodes present in its next level are left uncolored. The nodes in following level (i.e., grandchildren of $r$) are colored using colors $c_j$ where $j \not\in \{0,i\}$ and each of the nodes adjacent to each child of $r$ recieve a different color. Such an assignment is accomplished due to the fact that we have $\Delta - 1$ colors after coloring $r$ with $c_i$. This preserves the characteristic of \SH coloring by assigning at most $\Delta$ unique colors to the vertices in the closed neighborhood of each node of $T$. In other words, we color alternate levels of a tree to \SH color it. Therefore, either a vertex $v$ is colored or all its neighbors are colored using at most $\Delta$ colors.

\noindent
We remark that this may not be the optimal coloring in terms of number of colors used. However, this serves as an upper bound on the number of colors required to \SH color a tree.

\noindent
To prove the lower bound, consider a tree $T$ of height 2. Let $r$ be the root and $d$ be the number of children of each vertex in $T$, except leaves. Therefore, maximum degree $\Delta = d + 1$. Let $v$ be a vertex at height 1. Note that to \SH color the children of $v$, we need $d$ colors if we color each child of $v$ using a different color. Otherwise we have to color $v$ in order to dominate uncolored child node(s) of $v$. By extending this argument for each of $d - 1$ siblings of $v$, any \SH coloring of $T$ use $d$ colors. Thus the lower bound follows. Refer Figure \ref{Figure: label_sharTree}.

\end{proof}

\begin{figure}[htb]
\centering
\includegraphics[scale=0.7]{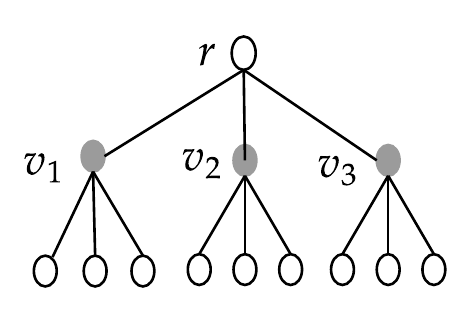}
\caption{\SH coloring tree $T$ with $d=3$}
\label{Figure: label_sharTree}
\end{figure}

\noindent
We observe that to \SH color tree $T$ in above construction requires $\Omega(\sqrt{n})$ vertices to be colored. Hence, we state the following corollary.

\begin{corollary}
There exist trees that require $\Omega(\sqrt{n})$ number of vertices to be colored so that the tree is \SH colored.
\end{corollary}

\noindent
Until now, we have explored the bounds for \SH coloring graph $G$ with respect to special graph classes, namely complete graph, path, cycle, threshold graph and trees. We will now examine \SH coloring with respect to some graph parameters. We consider the following graph parameters: maximum degree, treewidth, vertex cover size, cluster vertex deletion number, neighborhood diversity number and modular width. Note that the upper bounds for \SH coloring with respect to the said graph parameters are studied for a general graph $G$.

\subsection{Bounds for \SH coloring with respect to graph parameters}

\noindent
The first graph parameter that we study is the maximum degree $\Delta$ of graph $G$. Let us analyse the behavior of graph $G$ for \SH coloring with respect to $\Delta$.

\begin{lemma}
Let $\Delta$ be the maximum degree of a graph $G$. There exists a \SH coloring of $G$ such that $\chi_{ssc}(G)\leq\Delta^2+1$.
\end{lemma}
\begin{proof}
\noindent
For a given graph $G$, we construct graph $G^2$ as follows. The vertices $V(G^2)$ are same as vertices $V(G)$. We retain the edges of $E(G)$ in $E(G^2)$. Further, consider two non adjacent vertices $u$ and $v$ in $G$. If there exists a vertex $w$ that is adjacent to both $u$ and $v$, then add an edge $uv$ to graph $G^2$. This is done for every pair of distance-2 vertices $u$ and $v$ to get edge set of graph $G^2$. We observe that proper coloring of graph $G^2$ gives us a \SH coloring for graph $G$. Therefore, number of colors required to \SH color graph $G$ is $\chi(G^2) \leq \Delta^\prime + 1$, where $\Delta^\prime$ is the maximum degree of a vertex in $G^2$. Since $\Delta^\prime$ is at most $\Delta^2$, the result follows.

\end{proof}

\noindent
The next parameter of interest is the treewidth of graph $G$. Treewidth is a measure of how close a graph is to a tree-like structure. However, with respect to this parameter, it is uncertain to predict the behavior of \SH coloring when we try to capture the number of colors required for $G$. Consider the case of complete graphs. As described in Lemma \ref{completeG}, the number of colors required to \SH color a complete graph is 1. However, its treewidth is $O(n)$. On the other hand, we note that there exist trees, although the treewidth being 1, such that $\chi_{ssc}\geq\sqrt{n}$, as proved in Lemma \ref{treebound}. Let us now examine vertex cover as a parameter of $G$ which is larger then treewidth.

\begin{lemma}\label{sharVCbound}
The number of colors required to \SH color the vertices of graph G  is at most the size of vertex cover of $G$, that is, $\chi_{ssc}(G)\leq \textsc{VC(G)}$.
\end{lemma}

\begin{proof}
We know that every edge $e \in E(G)$ has at least one of its end vertices in vertex cover of $G$. Consider a graph $G$ with a vertex cover $X$ of size $k$. Firstly, assign one of the $k$ colors to all isolated vertices, if they exist. Next assign different colors to each vertex that form the vertex cover of $G$. Therefore, we have utilized $k$ colors to color vertices in $X$ as the size of $X$ is $k$. This \SH colors the vertices in $X$. By the definition of vertex cover of $G$, each edge $e \in E(G)$ has at least one of its end vertices in vertex cover and hence it is colored by one of the $k$ colors. Since we color each vertex of $X$, we are sure that vertices in $V(G)\backslash X$ will be adjacent to at least one of the colored vertices in $X$. Moreover, each vertex in $X$ is colored using a different color which avoids overlapping of colors. Therefore, we can conclude that every vertex $v \in V(G)$ has a colored vertex in its closed neighborhood. Further, in the presence of more than one colored neighbor, we can be assured of the color being distinct as all the vertices in $X$ as colored using $k$ different colors, hence satisfying \SH coloring of $G$.

\end{proof}

\noindent
We proceed to understand the nature of \SH coloring with respect to  the the size of cluster vertex deletion set of graph $G$ which is a smaller parameter compared to vertex cover of $G$.

\begin{definition}
A cluster graph is a disjoint union of complete graphs.
\end{definition}

\begin{definition}
A cluster vertex deletion set $X$ of a graph $G$ is a set of vertices such that $G\backslash X$ forms a cluster graph.
\end{definition}
\noindent
The cluster vertex deletion number is defined as the minimum possible size of cluster vertex deletion set $X$. Intuitively, it is the measure of how close a graph is to being a cluster graph.

\begin{lemma}\label{sharCVDSbound}
Let $X$ be a cluster vertex deletion set of graph $G$. Then $\chi_{ssc}(G)\leq |X|+1$.
\end{lemma}
\begin{proof}
To \SH color graph $G$, we color each vertex $v \in X$. If the size of $X$ is $k$, then we have utilized $k$ colors. Now color exactly one of the undominated vertices in each complete graph(s) in $G\backslash X$ using a color that is different from previously used $k$ colors. Note that two colored vertices $u$ and $v$ in two different cluster graphs do not have a common neighbor in $X$ because in such a scenario, we would not choose either of $u$ or $v$ to assign it the $(k+1)^{th}$ color. We assign $(k+1)^{th}$ color to an $undominated$ vertex in each cluster graph which implies that this vertex is not adjacent to any vertex in $X$. This gives us a \SH coloring of $G$ as the vertices in $X$ are dominated by the colors assigned to them. Additionally, some of the vertices in $G\backslash X$ may also have a neighbor in $X$. Every $v \in V(G)$ has at least one colored neighbor in $N[v]$ and in case more than one colored vertices are present in $N[v]$, we are assured of them being distinct because we have used $k+1$ colors. Therefore the result follows.
\end{proof}

\noindent
The next graph parameter for study of \SH coloring is the neighborhood diversity of $G$.

\begin{definition}
\cite{gargano2015complexity} Given a graph $G = (V,E)$, two vertices $u,v \in V$ have the same type if and only if $N(v)\backslash\{u\} = N(u)\backslash\{v\}$. The graph $G$ has a \textit{neighborhood diversity t}, if there exists a partition of $V$ into at most $t$ sets, $V_1, V_2,\dots,V_t$ such that all the vertices in $V_i$ have the same type for $i = 1,2,\dots,t$. The family $\nu = \{V_1,V_2,\dots,V_t\}$ is called the type partition of $G$.
\end{definition}
\noindent
On creating such a type partition of $V(G)$, we observe that the vertices within a partition either form a complete graph or an independent set. Further, for $1 \leq i, j \leq t$, each vertex in a partition $V_i$ is either adjacent to every vertex in another partition $V_j$ or there are no edges between vertices of $V_i$ and $V_j$.

\begin{lemma}\label{sharNDbound}
The number of colors required to \SH color a graph $G$ is at most its neighborhood diversity, that is, $\chi_{ssc}(G)\leq t$.
\end{lemma}
\begin{proof}
For a given graph $G$, consider its type partition $\nu$ with neighborhood diversity $t$. Color all isolated vertices, if any, using one of the $t$ colors. For $1 \leq i \leq t$, color a vertex in each $V_i$ using a different color. By doing so we \SH color $V(G)$. This can be justified as follows. Partitions $V_i$ that form a complete graph are all dominated due to the presence of a colored neighbor in $V_i$. Additionally, if vertices of $V_i$ are adjacent to partition $V_j$ for $1 \leq j \le t$, we can expect them to be adjacent to some more colored neighbors. Now consider the case where vertices in partition $V_i$ form an independent set. If vertices in partition $V_i$ are not isolated vertices, then they will be adjacent to all vertices of another partition $V_j$ which assures the presence of at least one colored neighbor in the closed neighborhood of each vertex in $V_i$. Hence we have used $t$ number of colors to \SH color $G$.
\end{proof}

\noindent
We conclude this section on bounds on the number of colors for \SH coloring by studying the problem for modular width of $G$. The modular width of graph $G$ is computed by virtue of four operations, namely creation of isolated vertex, disjoint union, complete join and substitution. More precisely, the modular width of $G$ equals the maximum number of operands used by any occurrence of  substitution operation. These four operations that are involved in modular decomposition of graph $G$ are described in \cite{modularwidth}. For the sake of completeness, we mention the four operations here.

\begin{definition}\label{mod_def} \cite{modularwidth} Algebraic operations involved to compute modular width of graph $G$.
\begin{itemize}
\item Create an isolated vertex;
\item The disjoint union of two graphs, i.e., the \textit{disjoint union} of two graph $G_1$ and $G_2$, denoted by $G_1 \otimes G_2$, is the graph with vertex set $V(G_1)\cup V(G_2)$ and edge set $E(G_1)\cup E(G_2)$;
\item The complete join of two graphs, i.e., the \textit{complete join} of two graphs $G_1$ and $G_2$, denoted by $G_1\oplus G_2$, is the graph with vertex set $V(G_1)\cup V(G_2)$ and edge set $E(G_1)\cup E(G_2)\cup \{ \{v, w\}: v\in V(G_1)$ and $w\in V(G_2)\}$.
\item The substitution operation with respect to some graph $G$ with vertices $v_1,\dots,v_n$, i.e., for graphs $G_1,\cdots,G_n$ the substitution of the vertices of $G$ by the graphs $G_1,\cdots,G_n$, denoted by $G(G_1,\dots,G_n)$, is the graph with vertex set $\underset{1 \leq i \leq n}\cup V(G_i)$ and edge set $\underset{1 \leq i \leq n} \cup E(G_i)\cup \{\{u, v\}:u \in V(G_i)$ and $v \in V(G_j)$, $v_i,v_j \in E(G)$ and $i\neq j\}$. Hence, $G(G_1,\cdots,G_n)$ is obtained from $G$ by substituting every vertex $v_i \in V(G)$ with the graph $G_i$ and adding all edges between the vertices of a graph $G_i$ and the vertices of a graph $G_j$ whenever $\{v_i, v_j\} \in E(G)$.
\end{itemize}
\end{definition}

\begin{definition} \cite{modularwidth} Let A be an algebraic expression that uses only the four operation as mentioned in Definition \ref{mod_def}. We define the width of A as the maximum number of operands used by any occurrance of the substitution operation in A. Modular width of graph G, denoted as mw(G), is the least integer m such that G can be obtained from such an algebraic expression of width at most m.

\end{definition}

\begin{lemma}
The maximum number of colors required to \SH color $G$ equals the modular width of the graph, that is, $\chi_{ssc}(G)\leq mw(G)$.
\end{lemma}
\begin{proof}
Let us now examine the maximum number of colors required to \SH color $G$ while we perform each of the above mentioned operations, in that sequence. On introducing an isolated vertex, we \SH color it by using one color. To dominate the vertices created as a result of disjoint union of vertices, we would require the maximum of all colors that was used in each component of disjoint sets. The complete join operation involves introducing edges between the two sets of vertices on which we intend to perform a complete join. Edges are introduced between every pair of vertices of the two sets of vertices, in addition to the existing edges. By using exactly two colors and coloring one vertex in each partition, we \SH color all vertices introduced thus far. Finally, we examine the fourth operation, that is substitution. In the substitution operation, we replace each vertex $v_i \in V(G)$ with the graph $G_i$ and adding all edges between the vertices of a graph $G_i$ and the vertices of a graph $G_j$ whenever $\{v_i,v_j\}\in E(G)$ \cite{modularwidth}. We color one vertex in each $G_i$. Besides the presence of colored neighbor(s) in $G_i$, a vertex may possibly be adjacent to another colored vertex in $G_j$. To \SH color $G$, we would then require the number of operands in this operation.
\end{proof}

\begin{figure}[htb]
\centering
\includegraphics[scale=0.6]{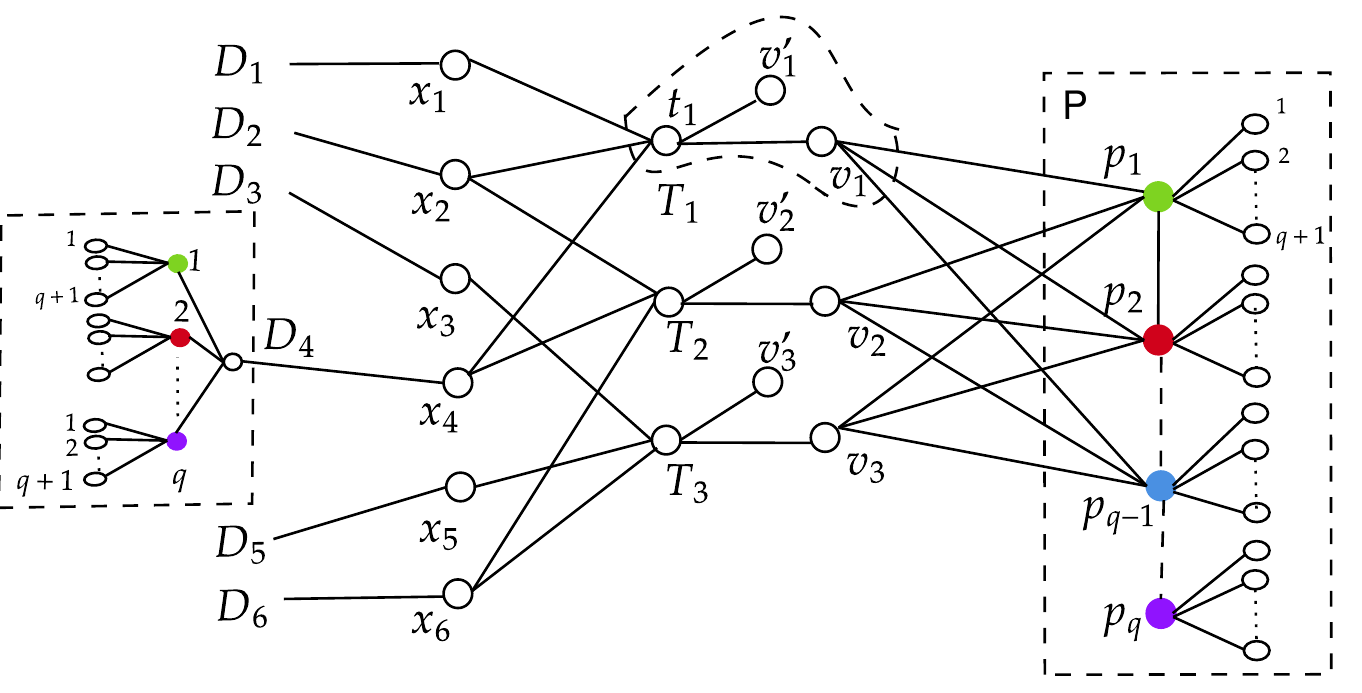}
\caption{\SH using $q$ colours on bipartite graph is also NP complete, where $q >2$.}
\label{kfull}
\end{figure}
